# Supplementary material for: NMR study of the Superconducting gap variation near the Mott transition in Cs$_{3}$C$_{60}$
Source: arXiv:1310.5529 source file (2014-02-19)
Supplement: Supplementary file 1 [file SCCs3C60_Suppl.pdf]

*Supplemental Information*

*for*

# NMR study of the Superconducting gap variation near the Mott transition in $Cs_3C_{60}$


P. Wzietek,[1] T. Mito,[1,2] H. Alloul,[1] D. Pontiroli,[3] M. Aramini,[3] and M. Riccò[3]

[1]*Laboratoire de Physique des Solides, Université Paris-Sud 11, CNRS UMR 8502, 91405 Orsay, France*

[2]*Graduate School of Material Science, University of Hyogo, Kamigori, Hyogo 678-1297, Japan*

[3]*Dipartimento di fisica e scienze della terra, Università di Parma - Via G.P.Usberti 7/a, 43100 Parma, Italy*



(Dated: December 2, 2013)

## A. SAMPLE

We present here in Fig.S1 the high resolution X-ray powder diffactogram and the quantitative analysis (QPA) performed by Rietveld refinement of the data [1], which allowed us to determine the $Cs_3C_{60}$ phases fractions. Those were found reproducible for different capillaries taken from the same sample batch.

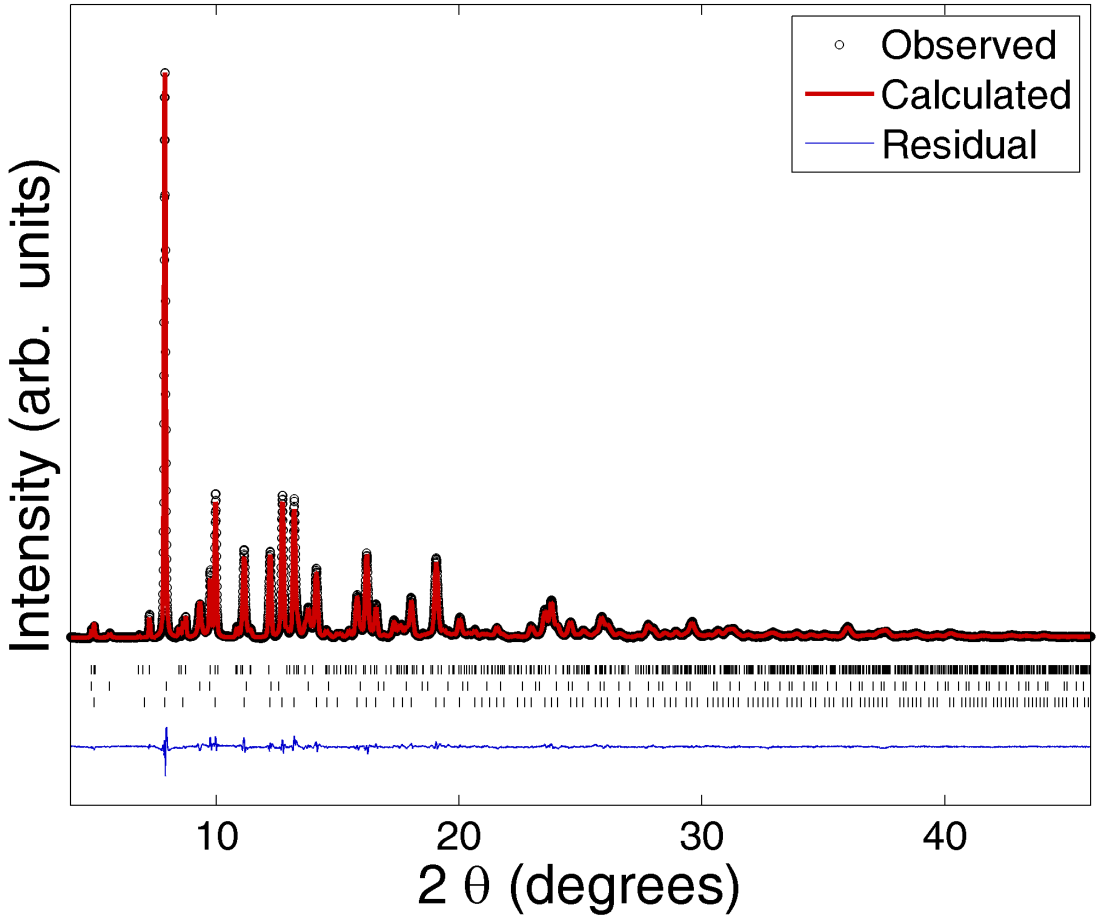


FIG. S1. X ray powder diffraction data of the sample collected at room temperature and ambient pressure at the beamline Cristal at Soleil ($\lambda = 0.72391(1)$ Å). The quantitative analysis performed by the Rietveld refinement of the data (Rwp = 4.25 %, RF2 = 5.88 %) permitted us to determine the following fractions of the three phases: 73(1) % of A15, 15(2) % of fcc and 12(1) % of bco.

The diamagnetic data presented in Fig. 1 of the main text permit us to locate the pressure of the transition from an insulator to the SC state at $p_c = 5.0 \pm 0.3$ kbar. The $T_c$ values measured with no applied field used to produce the phase diagram in Fig.1(c) have been determined as sketched in

Fig. 1(a), from linear extrapolations of the diamagnetic signals. The apparent experimental width of the transition might be associated with a distribution of pressures in the cell. Such average $T_c$ values differ from the onset values $T_c^{onset}$ (by as much as 1.5K at 5.9 kbar). As the data in Fig.1(b) correspond to $dT_c/dp = 3$ K/kbar in the investigated range above 5.1 kbar, the difference between the estimated average $T_c$ value and $T_c^{onset}$ would correspond to a maximum $0.5$ kbar width of the distribution of pressures in the cell, quite coherent with the detected width of the transition of $\pm 0.3$ kbar. This width could as well be due to a distribution of $p_c$ associated with sample defects.

The present $T_c$ values are slightly higher than our former results [2] obtained on a mixed phase sample with a larger fcc phase content. In [3] the reported $T_c$ data are even higher at comparable pressures although the transition width appears there much wider and their choice of $T_c^{onset}$ tends to overestimate $T_c$ with respect to that used here.

The data for our sample are therefore defining a sharp transition which appears as first order and is better delineated than in all the former published data [2, 3] evaluated so far mostly from the diamagnetic fraction measured in mixed phase samples. This homogeneous sample has been essential in allowing us to follow by NMR the evolution of the electronic properties in both metallic and SC states close to the Mott transition.

### B. NMR SPECTRA

All $^{133}$Cs and $^{13}$C NMR measurements have been carried at the same magnetic field $H = 8$ T. At this field the $T_c$ values as obtained from the NMR shifts and the relaxation rate are about 1.5 K lower than those obtained by diamagnetic measurements.

The intensity ratio between the $^{133}$Cs NMR signals of the fcc and the A15 phase can be reduced by a factor 3 using adequate spin echo sequence, as has been detailed in [2]. So, given the relative phase content given by the X ray Rietveldt analysis, the spectra shown in Fig. S2 are those for an A15 sample contaminated by by at most (1/3) (15/73) that is $\sim 7\%$ of the fcc phase signal. In Fig. S2, we indeed could not distinguish above $T_c$ any such contribution of the fcc phase to the NMR signal. However for the long repetition times used in the reported spectra the contribution of the insulating $Cs_4C_{60}$ phase for which the spin contribution to the $^{133}$Cs shift is small can be seen on the left of the spectrum around -15 kHz (this contributes to the non symmetric aspect of the spectrum). In any case, as the NMR signal of this phase is shifted on the left of the A15 signal, it only slightly contaminates the right hand side of the A15 spectrum which has been used

to determine the $^{133}$Cs relaxation rates.

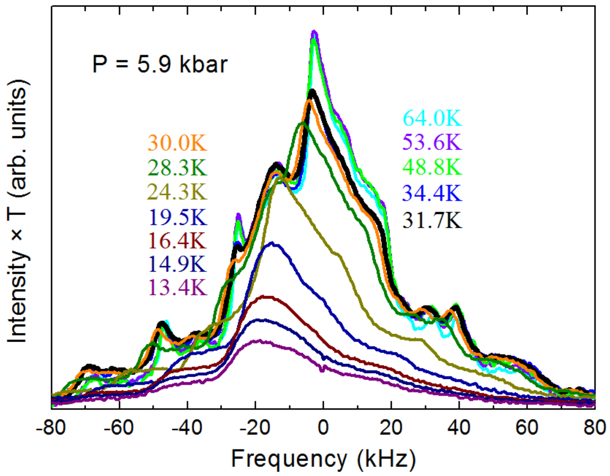


FIG. S2. The $^{133}$Cs spectra measured at $H = 8$ T, $p = 5.9$ kbar for various temperatures above and below $T_c$. Notice that the spectra, normalized by $1/T$ to correct for the Curie increase of nuclar spin magnetization, are quite identical above $T_c$ but shift and broaden in the SC state as can be expected.

The spectra displayed in Fig. S2 were collected at 5.9kbar for which the sample is fully metallic and SC. As can be seen, no modification of the spectrum shape happens down to $T_c \sim 30$ K. (Note that at lower pressures a partial loss of intensity on the right part of the signal is detected at the Nel temperature $T_N = 47$ K and signals the occurence of a contibution to the signal of a significant fraction of coexistent AF A15 phase. This will be detailed in a forthcoming publication.)

In the SC state, the penetration of vortices and the associated screening currents induce a shift and a broadening of the NMR signal. The significant shifts analysed hereafter in the Fig.Fig. S4 of section C2 are due to the reduction of the spin susceptibility in the paired state. This is a signature of the singlet nature of the SC state in these compounds, which we already evidenced in [2] for data taken ar higher pressures.

## C. ANALYSIS OF THE $^{13}$C NMR SPECTRA

The NMR shift of a nuclear spin site is a tensor $K^{\alpha}$ where $\alpha$ is related to the orientation of the applied magnetic field with respect to the local crystallographic axis on the corresponding site. The isotropic component $K^{iso} = (1/3)\sum K^{\alpha}$ induces a shift of the first moment of the spectrum. In powder samples, any anisotropic contribution to $K^{\alpha}$ induces a broadening of the NMR signal

with a shape defined by the anisotropic tensor (as that seen for instance above $T_c = 30$ K in Fig.2(a) of the main text).

To analyze the spectra we consider the three contributions listed in Eq.1 of the main text: $K^{\alpha}_{orb}$, $K^{\alpha}_{s}$, and $K_{dia}$, the last two being $T$ dependent in the SC state.

The isotropic term $K_{dia}$, specific to the SC state, is the inhomogeneous diamagnetic reduction ($K_{dia}H$) of the field sensed by the nuclei, resulting from the macroscopic screening currents and the vortices. The orbital contribution $K^{\alpha}_{orb}$, due to the atomic or molecular orbital currents associated with filled electronic shells is usually $T$ independent even through the SC transition. The electronic metallic properties are probed by the Knight shift, that is the spin part of the NMR shift $K^{\alpha}_{s} = A^{\alpha}\chi_s(T)$, where $A^{\alpha}$ is the hyperfine coupling tensor and $\chi_s(T)$ the spin susceptibility which vanishes at $T = 0$ for a singlet SC state.

### C.1. Anisotropic contribution

The modification of the $^{13}$C spectrum shape below $T_c$ is primarily associated with a rapid variation of the anisotropic contribution to $K^{\alpha}$, which even changes sign below $T_c$. This is well known for metallic $A_n$C$_{60}$ compounds [4], as the unpaired electronic spins are in the $t_{1u}$ molecular orbitals, which are hybridized $p - \pi$ carbon orbitals orthogonal to the C$_{60}$ sphere. The latter couple mainly with the $^{13}$C nuclear spin by the anisotropic electron-nucleus dipole-dipole interaction [2, 4], which is expected to give an axial shift anisotropy. Here we assumed that $K^{ax}_{s}$ and $K^{ax}_{orb}$ have the same principal axes. Therefore the spin and orbital shift tensor components are ($K^{c} = K^{iso} + K^{ax}, K^{ab} = K^{iso} - K^{ax}/2$) in the triad reference frame orthogonal to the C$_{60}$ ball on a $^{13}$C site.

The orbital term $K^{\alpha}_{orb}$ is the unique contribution to the $^{13}$C NMR shift in non metallic $A_n$C$_{60}$ compounds, such as pure C$_{60}$ itself [5], or Na$_2$C$_{60}$ and K$_4$C$_{60}$ [6], which are electronically charged Mott Jahn-Teller insulators with no spin susceptibility contribution [6]. The comparison of those cases leads us to consider that $K^{ax}_{orb} \sim -120$ ppm can be legitimately taken for A15-Cs$_3$C$_{60}$.

To analyze the data below $T_c$, it is necessary to consider also the diamagnetic contribution $K_{dia}$ (related to the SC properties through the penetration and coherence lengths), which induces an additional broadening of the spectrum which increases progressively below $T_c$. The fit of our lower $T$ spectrum using $K^{ax}_{orb} = -120$ ppm, and assuming that $\chi_s(T)$ and therefore $K^{ax}_{s}(T)$ have nearly vanished at 15 K, allowed us to estimate that the low temperature field distribution associated with

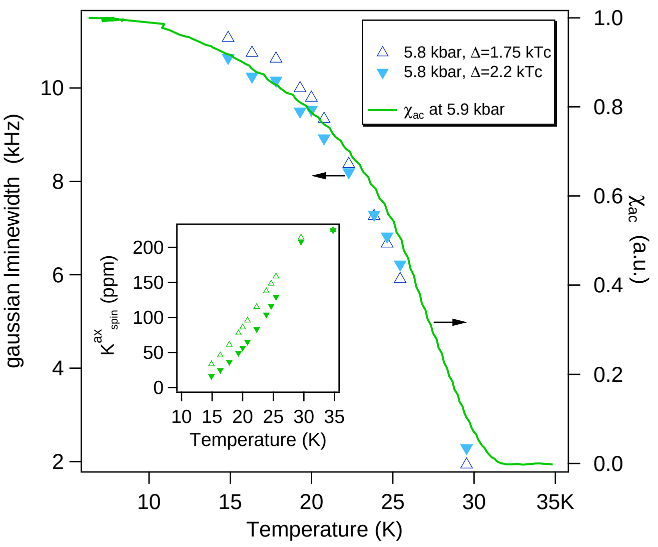


FIG. S3. Gaussian linewidths (main panel, left scale) in the SC state as obtained by fits of the spectra for two distinct variations of $K_s^{ax}(T)$ (inset). The fits are as good for a weak coupling BCS ($\Delta = 1.75kT_c$, empty symbols) or a larger gap value ($\Delta = 2.2kT_c$, full symbols). The variation of the linewidths is found similar to that of the zero-field diamagnetism (full line,right scale, also Fig. 1 of the main text).

$K_{dia}$ can be very well modeled by a gaussian shape. Therefore three parameter fits permit us to get $K^{iso}(T)$ and $K^{ax}(T)$ almost independently from the gaussian linewidth ($K^{iso}$ obtained from the fit is in perfect agreement with that obtained from the first moment of the spectra). However such a temperature dependent gaussian broadening superimposed over the anisotropic spectrum reduces the accuracy in the determination of $K^{ax}(T)$, especially in the region slightly below $T_c$ where $K_s^{ax}$ and $K_{orb}^{ax}$ nearly balance each other. As shown in Fig. 2(a) of the main text, we could fit the spectral shapes by imposing a variation of $K_s^{ax}(T)$ similar to that expected for a BCS singlet state SC. But, as shown in Fig. S3, the data can be fitted as well either assuming a BCS singlet Yosida function with the BCS gap or with a larger gap value of $\Delta = 2.2kT_c$, at the expense of slight modification of the magnitude of gaussian broadening.

In conclusion, this analysis of the $^{13}$C spectral shapes permits us to ensure the overall consistency with a singlet state SC behaviour but does not allow to decide whether the gap magnitude is increased with respect to a BCS gap.

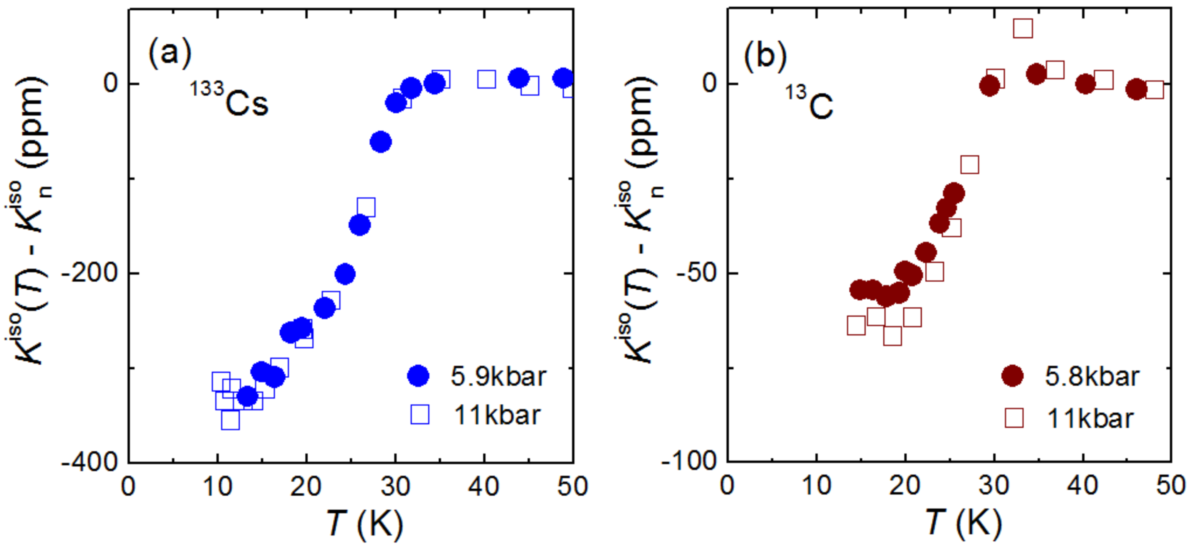


FIG. S4. Isotropic shift of the $^{133}$Cs and $^{13}$C spectra measured at 5.9 kbar (respectively 5.8 kbar) and 11 kbar for various temperatures above and below $T_c$. The data for $^{133}K_{iso}$ versus T are deduced from the spectra of Fig. S2

### C.2. Isotropic shifts

The value of $^{13}K^{iso}(T)$ obtained from the fits are reported in Fig.S4(a). In Fig.S4(b) we also show $^{133}K^{iso}(T)$ obtained from the spectra of Fig. S2. There, though an asymmetry of the central line points out a small anisotropy of the shift in the normal state, the data for $^{133}K^{iso}(T)$ have been taken from the Fig. S2 spectra at the peak of the central line position. As long as the broadening due to the distribution of $K_{dia}$ is rather small, that is down to $T \sim 25$K (see Fig. S3), this permits to monitor reliably the sharp initial drop of $^{133}K^{iso}(T)$ which occurs just below $T_c$. At lower temperatures the uncertainty on $^{133}K^{iso}$ is mostly determined by the increased linewidth associated with the distribution of $K_{dia}$.

The spin susceptibility $\chi_s(T)$ can also be determined from these isotropic shifts, provided we can determine and subtract the isotropic part of $K_{dia}$. This can be done using $K^{iso}$ measured at the same magnetic field for both the $^{13}$C and $^{133}$Cs nuclei [4]: the fields induced by the screening currents do not depend on the nuclear probe and thus $K_{dia}$ is eliminated in $\Delta K^{iso} \equiv ^{133} K^{iso} - ^{13} K^{iso}$, which therefore reflects the variation of $\chi_s(T)$ below $T_c$ :

$$\Delta K^{iso} = ^{133} K^{iso}_{orb} - ^{13} K^{iso}_{orb} + (^{133}A^{iso} - ^{13} A^{iso}_s)\chi_s(T) \tag{1}$$

The variation of $\Delta K^{iso}(T)$ taken at 5.9 kbar (and neglecting the 0.1 kbar pressure difference

between the $^{13}$C and $^{133}$Cs data sets) is plotted in Fig.2b of the main text.

## D. SPIN LATTICE RELAXATION DATA

### D.1. Nuclear magnetization recovery shapes

Nuclear spin lattice relaxation times have been obtained by monitoring the recovery of the nuclear magnetization, which can be fitted with a stretched exponential recovery

$$M_0 - M(t) = M_0\left(\exp(-t/T_1)\right)^{\beta}. \tag{2}$$

as can be seen in Fig S5.

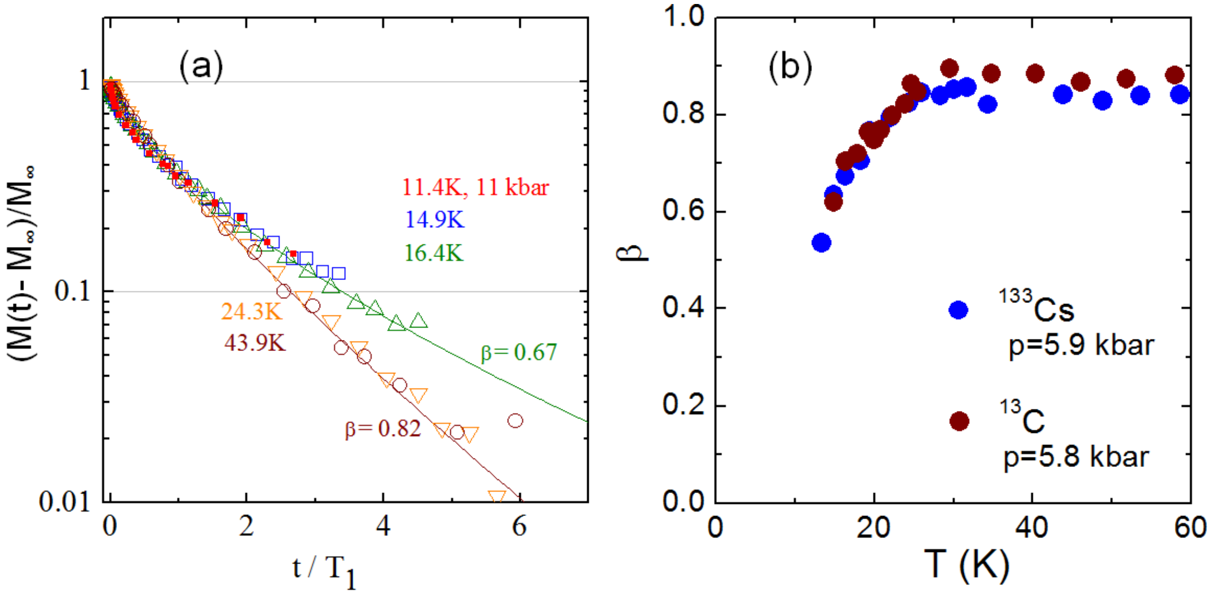


FIG. S5. (a) Variation of the $^{133}$Cs nuclear magnetization recovery profiles for various temperatures above and below $T_c$ measured at 5.9 kbar. Fits with the stretched exponential function are displayed. (b) The variation with temperature of the fitted stretched exponents $\beta$ are quite similar for $^{13}$C and $^{133}$Cs.

In the normal state the stretched exponent are found nearly temperature independent, with $\beta \simeq 0.8$ for the two nuclear species. For the $^{133}$Cs nuclei the relaxation curves were obtained integrating the higher half of the Cs spectrum to avoid any contribution due to the $^{133}$Cs NMR signals of the $Cs_4C_{60}$ or fcc-$Cs_3C_{60}$ which both occur on the left side of the spectrum. Below $T_c$ the exponent $\beta$ slightly diminishes so that a larger distribution of relaxation rates occurs in the SC state. We

limited our data down to $\sim$ 11K, that is $\sim T_c/3$. At lower temperatures the measurements become more difficult due to the loss of the NMR signal intensity (determined by rf penetration) and long $T_1$'s. In fact $T_1$ becomes so long at those temperatures that the time dependence of the magnetization recovery becomes then different from that in the normal state. The recovery profile acquires a different stretched exponent presumably because defects and motion of vortices contribute to the distribution of $T_1$. However the observed deviations at low $T$ have little impact on the gap determination obtained from the $T_1$ measurements.Indeed, we show in Fig. S5 that the observed deviations at low $T$ correspond to a decrease of the relaxation rate for a small fraction of the nuclear spins. So the reported relaxation time in the stretched exponent is shorter than that which one would obtain by taking an average of $1/T_1$ on all sites. In other words this reduction of the exponent $\beta$ consequently leads us to estimate an upper limit of the $1/T_1$ value. If one were to put error bars on the low T data of Fig. 3(a) or (b) of the main text, those would extend toward lower $1/T_1$ at low $T$, which would even yield larger SC gap values.

### D.2. Hebel-Slichter coherence peak

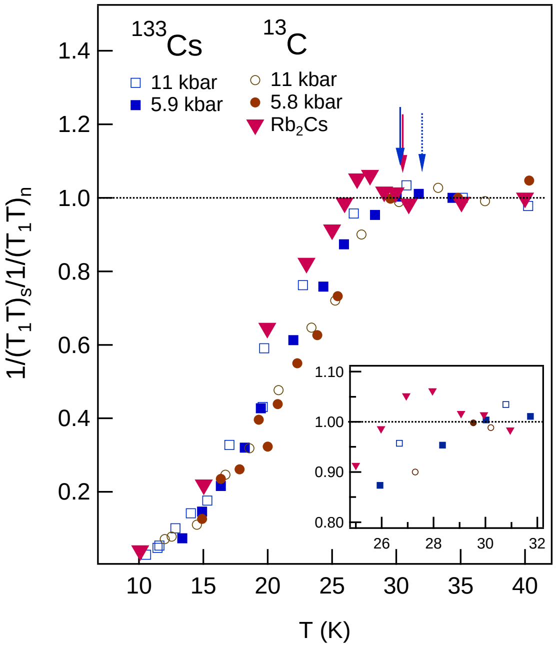


FIG. S6. $1/(T_1T)$ normalized to the normal state value (zoom in the inset). The data for $Rb_2CsC_{60}$ is taken from [4]. The arrows indicate the $T_c$ values.

In Fig. S6 we show the variation of $1/(T_1T)$ corresponding to the data of the figure 3 of the main text. The data for the two nuclear spin species and the two pressures are normalized to the value at 35 K. For comparison we show the corresponding data for $Rb_2CsC_{60}$ obtained at $H = 8.8$ T [4]. The latter shows a slight increase below $T_c$ which has been interpreted as a Hebel-Slichter peak partly suppressed by the magnetic field [4]. The interesting feature of our results is that there is no sign of such effect at 5.8 kbar for all our data (a vestigial effect might be present at 11 kbar). Here the comparison is meaningful as all data were obtained in a similar magnetic field. Therefore, our results reveal that the Hebel-Slichter peak is suppressed when approaching the Mott transition on the left side of the SC dome.

*Acknowledgements.* We would like to thank S. Ravy and E. Elkam for helping us to perform this sample test at the CRISTAL beam line at SOLEIL in an experiment preparatory to high pressure proposals done later.

---

[1] D. L. Bish and S. A. Howard, Journal of Applied Crystallography **21**, 86 (1988).

[2] Y. Ihara, H. Alloul, P. Wzietek, D. Pontiroli, M. Mazzani, and M. Riccò, Phys. Rev. Lett. **104**, 256402 (2010).

[3] Y. Takabayashi, A. Y. Ganin, P. Jeglic, D. Arcon, T. Takano, Y. Iwasa, Y. Ohishi, M. Takata, N. Takeshita, K. Prassides, and M. J. Rosseinsky, Science **323**, 1585 (2009).

[4] C. H. Pennington and V. A. Stenger, Rev. Mod. Phys. **68**, 855 (1996).

[5] R. Tycko, G. Dabbagh, R. M. Fleming, R. C. Haddon, A. V. Makhija, and S. M. Zahurak, Phys. Rev. Lett. **67**, 1886 (1991).

[6] V. Brouet, H. Alloul, S. Garaj, and L. Forró, Phys. Rev. B **66**, 155122 (2002).
